# Supplementary material for: Local migration quantification method for scratch assays
Source: arXiv:1806.09219 ancillary file (2018-06-24)
Supplement: Supplementary file 1 [file supporting_information.pdf]

# Supporting Information

## 1 Objective function for optimal window size

We describe the objective function to calculate the optimal window size in detail. Let us consider a window size $w$ and divide $Y$, which has size $D$, into $M = D/w$ segments $Y_s$ of length $w$. $Y_s$ is the set of pixels that belong to a segment of length $w$. When $D$ is not divisible by $w$, $Y$ is divided into $M = \left\lfloor \frac{Y}{w} \right\rfloor + 1$ segments, where the first $\left\lfloor \frac{Y}{w} \right\rfloor$ segments have length $w$ and the last one, has length $D - w \times \left\lfloor \frac{D}{w} \right\rfloor$. After applying the linear approximation with respect to the window size $w$, we have the following approximation for the interface position at time $t_n$ for each $j \in Y_s$,

$$i_j(t_n) \approx m_s t_n + b_s, \tag{1}$$

where $m_s$ and $b_s$ are determined as described in Section 2.4. We consider the following fitness functions that evaluate the interface position approximation (1):

1. Residual sum of squares
$$E(w) = \frac{1}{2D} \sum_{j=1}^{D} \left( {e_l}_j^2 + {e_r}_j^2 \right) \tag{2}$$
where $e_{li} = i_j(t_n) - (m_s t_n + b_s)$ is the residual squared of the position approximation (1) at time $t_n$. The subscript denotes the interface (left or right).

2. Linear fitness
$$R(w) = \frac{1}{2D} \sum_{j=1}^{D} {R_l}_j^2 + {R_r}_j^2 \tag{3}$$
where ${R_l}_j^2$ is the coefficient of determination $R^2$ of the $j$-th coordinate of the left interface height approximation (Equation 1). The better the linear fit, the closer $Fit_{R^2}$ should be to 1. The subscript denotes the interface (left or right).

3. Fitness between left and right velocities
We consider a distance metric derived from the Kolmogorov-Smirnov test statistic (Bonamente, 2013). Given two data sets $\{a_s\}_{s=1}^n$ and $\{b_r\}_{r=1}^m$ and $F_n$ and $F_m$ their empirical cumulative distributions, respectively, the Kolmogorov-Smirnov statistic is:
$$D_{n,m} = \sup_{x \in \mathbb{R}} |F_n(x) - F_m(x)|. \tag{4}$$
Normalizing the statistic by the effective number of data points, we obtain the KS distance that was introduced in Fabbri and De León (2017):
$$Dist(\{a_s\}_{s=1}^n, \{b_r\}_{r=1}^m) = \frac{nm}{n+m} D_{n,m}, \tag{5}$$
where $\{a_s\}_{s=1}^n$, $\{b_r\}_{r=1}^m$ are two ordered data points. We consider the $KS_{distance}$ between the left and right windowed velocity distributions
$$KS_{distance}(w) = Dist\left(\{m_l\}, \{m_r\}\right), \tag{6}$$
where the subscripts denote the left and right side, respectively. Ideally, the left and right windowed velocity distribution should be the smallest possible.

We consider the following global function:

$$F(w) = Fit_{resid}(w) + Fit_{Rsquared}(w) + Fit_{KS_{distance}}(w), \tag{7}$$

where

$$Fit_{resid}(w) := \frac{E(w) - \min\limits_{1\leq w\leq D} E(w)}{\max\limits_{1\leq w\leq D} E(w) - \min\limits_{1\leq w\leq D} E(w)},$$

$$Fit_{Rsquared}(w) := \frac{R(w) - \min\limits_{1\leq w\leq D} R(w)}{\max\limits_{1\leq w\leq D} R(w) - \min\limits_{1\leq w\leq D} R(w)}, \tag{8}$$

and

$$Fit_{KS_{distance}}(w) := \frac{\max\limits_{1\leq w\leq D} KS_{distance}(w) - KS_{distance}(w)}{\max\limits_{1\leq w\leq D} KS_{distance}(w) - \min\limits_{1\leq w\leq D} KS_{distance}(w)}$$

The global fitness function is normalized such that $0 \leq Fit_{global}(w) \leq 1$ and the window with the largest value will be the optimal value with respect to the three fitness functions, weighted equally through the global function. The terms have been normalized so each term is between 0 and 1 and the largest value is the one maximizing each criteria.

If additional scratches are considered to calculate the optimal window, we consider a weighted sum of objective functions for each of the scratches considered. The objective function would be

$$F(w) = \frac{1}{S}\sum_{s=1}^{n} F_s(w), \tag{9}$$

where $F_s$ is the individual objective function for scratch assay $s$ and $S$ is the number of scratch assays considered.

# 2 Classification tests using in-silico data

We present the results of the classification tests for the three quantification methods with respect to the focal parameter $\hat{P}$ with values in $\{0.1, 0.5, 0.9\} \times \{0.01, 0.09\}$. We consider $n = 4$ simulations as the sample size for our test and repeat the classification test 20 times.

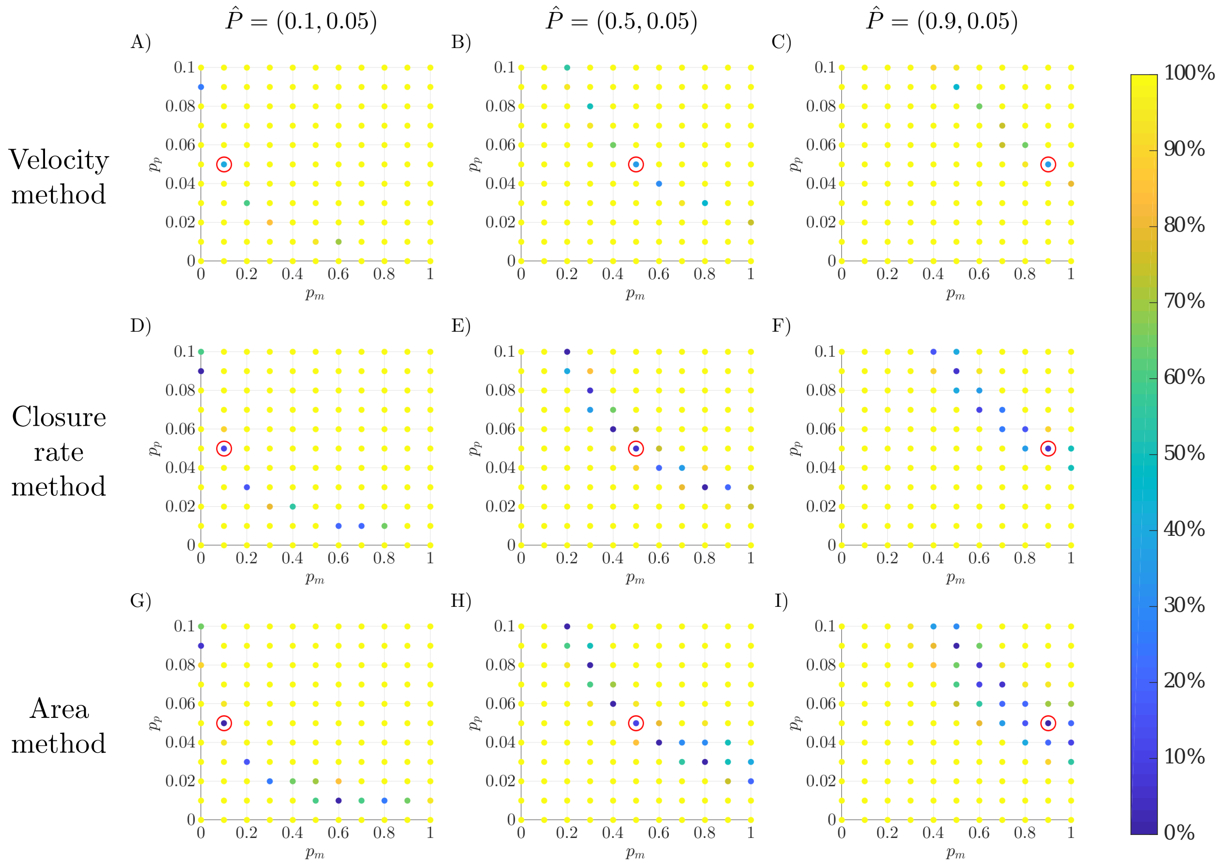


Figure 1: Series of plots showing how the performance of the three quantification methods changes as the motility rate of the focal parameters varies with fixed proliferation probability $\hat{p}_p = 0.01$. In each plot, the color of the circle at each parameter pair $(p_m, p_p)$ indicates the percentage of times the migration measurements associated with the parameter pair are statistically significantly different from those associated with the focal parameters $\hat{P}$. The focal parameters $\hat{P}$ are indicated by a red circle. The results reveal that the velocity method yields a better statistical classification than the other methods. We note also the performance of all three methods declines as the motility rate of the focal parameters $\hat{P}$ increases.

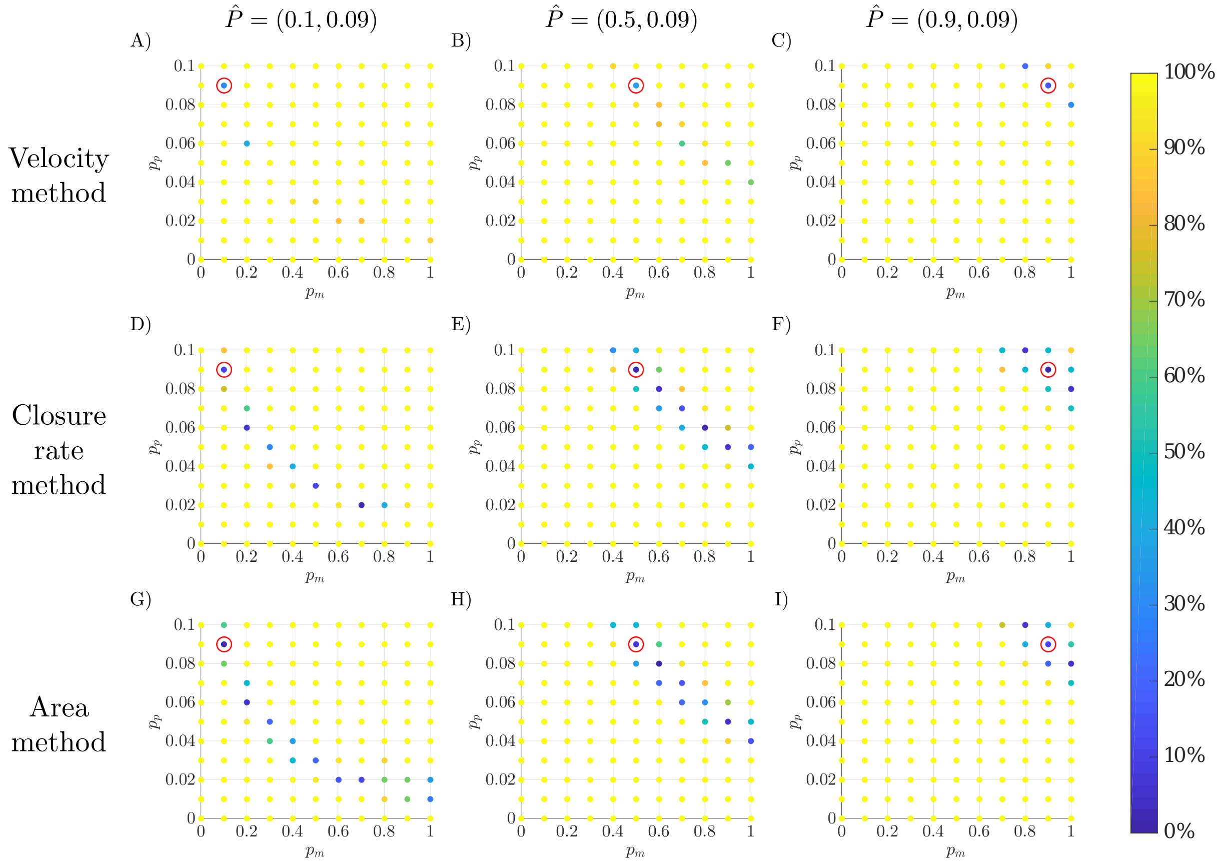


Figure 2: Series of plots showing how the performance of the three quantification methods changes as the motility rate of the focal parameters varies with fixed proliferation probability $\hat{p}_p = 0.09$. In each plot, the color of the circle at each parameter pair $(p_m, p_p)$ indicates the percentage of times the migration measurements associated with the parameter pair are statistically significantly different from those associated with the focal parameters $\hat{P}$. The focal parameters $\hat{P}$ are indicated by a red circle. The results reveal that the velocity method yields a better statistical classification than the other methods. We note also the performance of all three methods declines as the motility rate of the focal parameters $\hat{P}$ increases.

# 3 Determination of the optimal window size of the in-vitro data

We present the plots of the objective function and the three fitness functions that contribute to its calculation, applied to the in-vitro data.

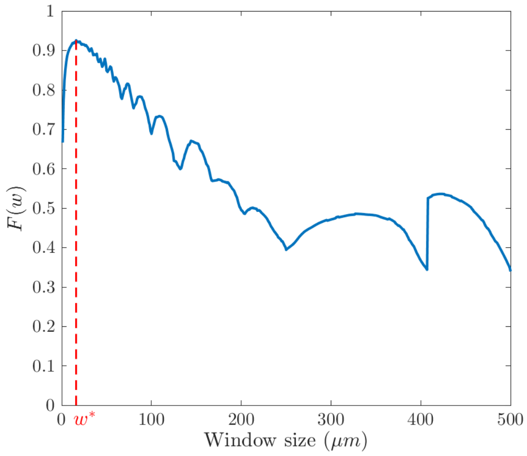


Figure 3: Plot of the objective function for the in-silico data. The optimal window size, $w^* = 16$ $\mu$m is indicated with a dashed line in red.

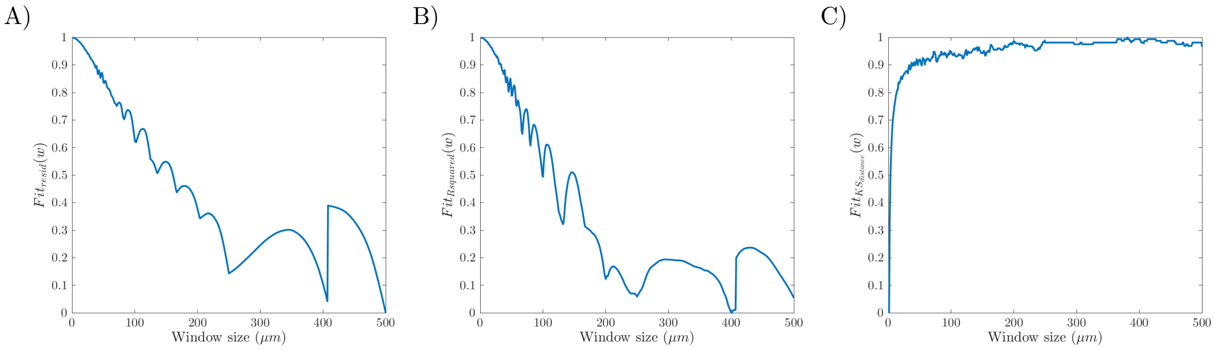


Figure 4: Plot of the fitness functions that constitute the objective function: A) $Fit_{resid}$, B) $Fit_{Rsquared}$ and C) $Fit_{KS_{distance}}$. The functions have been rescaled so their values are between 0 and 1.

# 4 Autocorrelation function of windowed velocities from in-silico data

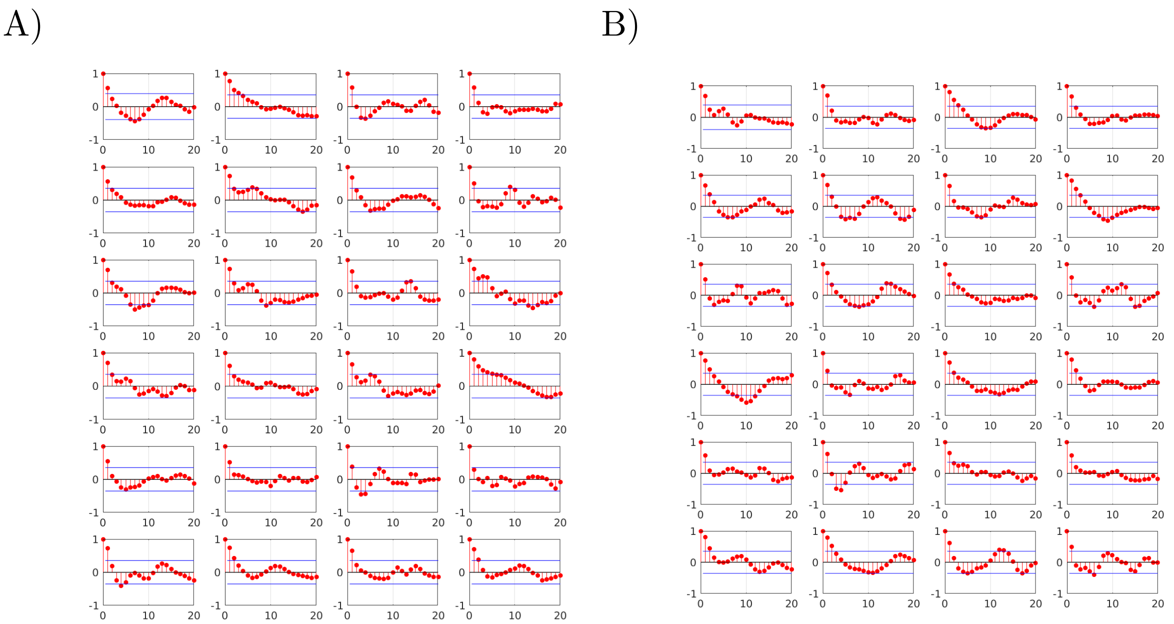


Figure 5: Autocorrelation functions of the A) left and B) right windowed velocities for the optimal window size $w^* = 16$ $\mu$m of each in-vitro scratch assay. The vertical axis is $lag\ \tau$ while the horizontal axis is the correlation coefficient $\rho(\tau)$ with respect the lag $\tau$.

# 5 Statistical classification of the in-vitro data

We present the results of performing the unpaired two-sample t-test (t-test), the Wilcoxon rank-sum test and the two-sample Kolmogorov-Smirnov test (K-S test) between the migration measurements of the S1 group against the other groups' measurements. We fix a $p$-value $< 0.05$ to define statistical significance. We indicate in each row the statistical test performed and in each column we indicate if the hypothesis was rejected ($h = 1$) or not ($h = 0$) and the corresponding p-value for each of the hypothesis test.

| | S2 | S3 | S4 | S5 | S6 |
|---|---|---|---|---|---|
| t-test | h=1, p=1.101e-07 | h=1, p=3.489e-46 | h=1, p=5.102e-27 | h=0, p=3.822e-01 | h=0, p=1.026e-01 |
| Wilcoxon rank sum test | h=1, p=3.626e-09 | h=1, p=7.146e-41 | h=1, p=4.907e-25 | h=0, p=3.401e-01 | h=0, p=4.520e-01 |
| K-S test | h=1, p=4.026e-09 | h=1, p=1.668e-33 | h=1, p=5.865e-18 | h=0, p=1.041e-01 | h=1, p=1.093e-02 |

Table 1: Hypothesis test results comparing S1 and the other group's windowed velocities. In each row the statistical test performed is indicated.

| | S2 | S3 | S4 | S5 | S6 |
|---|---|---|---|---|---|
| t-test | h=0, p=1.199e-01 | h=0, p=6.562e-02 | h=0, p=1.291e-01 | h=0, p=8.490e-01 | h=0, p=7.062e-01 |
| Wilcoxon rank sum test | h=0, p=3.429e-01 | h=1, p=2.857e-02 | h=0, p=2.000e-01 | h=0, p=6.857e-01 | h=0, p=3.429e-01 |
| K-S test | h=0, p=1.075e-01 | h=1, p=1.107e-02 | h=0, p=1.075e-01 | h=0, p=5.344e-01 | h=0, p=1.075e-01 |

Table 2: Hypothesis test results comparing S1 and the other group's closure rates. In each row the statistical test performed is indicated.

The evolution of the percentage wound area of each scratch assay during the course of the experiment is shown in Figure 6.

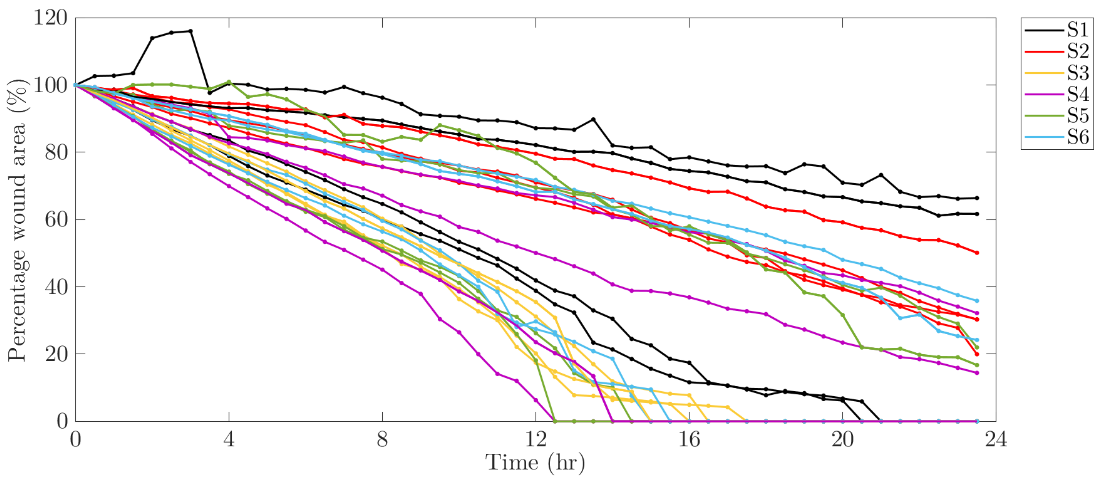


Figure 6: Evolution of the percentage wound area during the course of the experiment of each scratch assay. Experiments of the same cell group are plotted with the same color.

We calculated the time of comparison for the different groups, the results are presented in Table 6.

| | S2 | S3 | S4 | S5 | S6 |
|---|---|---|---|---|---|
| Time of comparison (hr) | 21 | 15 | 13 | 13 | 15 |

Table 3: Comparison times for the wound percentage areas of the different groups. The time of comparison was set to be half the time it takes for the first scratch being compared in which the leading edges touch.

The wound percentage area at the comparison times are shown in Figure 7.

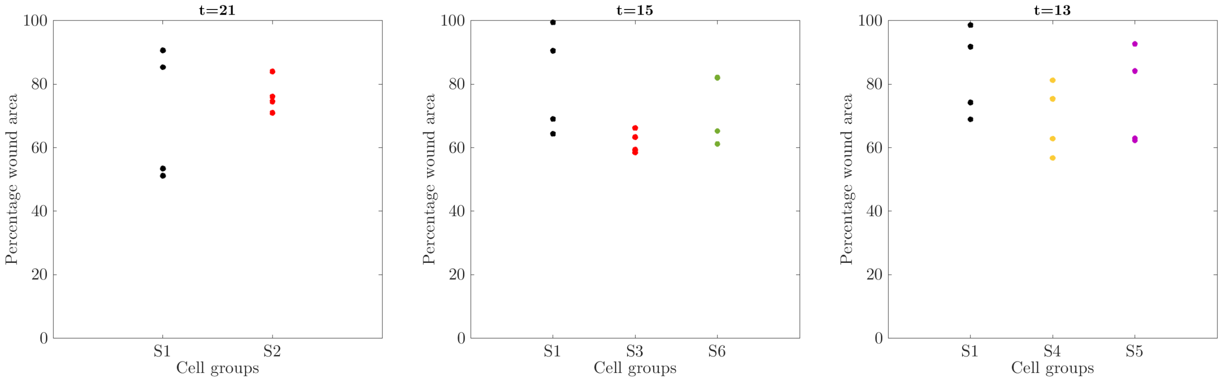


(a) $t = 21$ hr (b) $t = 15$ hr (c) $t = 13$ hr

Figure 7: Percentage wound area between S1 and the other groups at the time of comparison

The results of the statistical tests applied to the percentage wound area at the time of comparison are shown in Table 4.

| | S2 | S3 | S4 | S5 | S6 |
|---|---|---|---|---|---|
| t-test | h=0, p=5.819e-01 | h=0, p=6.936e-02 | h=0, p=1.632e-01 | h=0, p=4.790e-01 | h=0, p=4.447e-01 |
| Wilcoxon rank sum test | h=0, p=1.000e+00 | h=0, p=5.714e-02 | h=0, p=3.429e-01 | h=0, p=4.857e-01 | h=0, p=4.857e-01 |
| K-S test | h=0, p=5.344e-01 | h=0, p=1.075e-01 | h=0, p=5.344e-01 | h=0, p=5.344e-01 | h=0, p=5.344e-01 |

Table 4: Hypothesis test results comparing S1 and the other group's percentage wound areas. In each row the statistical test performed is indicated.

# References

Bonamente, M. (2013). *Statistics and analysis of scientific data*. Springer.

Fabbri, R. and De León, F. G. (2017). A statistical distance derived from the kolmogorov-smirnov test: specification, reference measures (benchmarks) and example uses. *arXiv preprint arXiv:1711.00761*.
